# Supplementary material for: GTAutoAct: An Automatic Datasets Generation Framework Based on Game Engine Redevelopment for Action Recognition
Source: arXiv:2401.13414 source file (2024-01-24)
Supplement: Supplementary file 1 [file X_suppl.tex]

\clearpage
\setcounter{page}{1}
\maketitlesupplementary

\section{Full Paper with Appendix}
\label{sec:rationale}
We have included the complete paper along with an appendix under the file name \textbf{``paper\_with\_appendix.pdf''} to offer further details about our work. 
Please note that the main content of the paper remains identical to that of the version initially submitted.

\section{Project Code}
The complete project code for GTAutoAct is accessible via an anonymous link for a private GitHub repository, which can be found here: \href{https://anonymous.4open.science/r/GTAutoAct-4CB6/README.md}{``Project code''}. 

\section{Data}
Due to the license agreements concerning the use of the Human3.6M, NTU RGB+D, and H3WB datasets, we are unable to distribute any datasets derived from these sources. 
This restriction includes all H36M-based datasets such as H36M-Original, H36M-Single, H36M-Extracted, H36M-SingleExtracted, H36M-Original-Test, and H36M-Segment-Test, as well as any NTU-based datasets, including NTU-Original and NTU-Test.
However, we offer the scripts needed to generate these datasets from the original sources, and these can be accessed and downloaded from the Project code repository as well.
Additionally, the datasets generated by GTAutoAct are available for download through an anonymous link to a private Google Drive. The link can be found here: \href{https://drive.google.com/drive/folders/1rZm-IZT45KjDLVDC3C_qOn7IPGVokPKH?usp=drive_link}{``Datasets''}.

\section{Reproducibility of Experiment}
In our paper, we perform a series of experiments on various action recognition models to assess the effectiveness of our method. To facilitate the reproduction of our results, we offer the following instructions.
For detailed information, please refer to the \textbf{``README.md''} attached with testing code.

\subsection{Experiment Setup}
We suggest utilizing MMAction, an open-source toolbox designed for video understanding, which is based on the PyTorch framework.
For setting up MMAction, please follow the setup instructions available on its \href{https://github.com/open-mmlab/mmaction2}{official GitHub repository}. 
For reference, the details of our experimental environments are outlined in Section B.1. of the appendix.

\subsection{Data Preparation}
Regarding the Human3.6M dataset, please refer to \href{http://vision.imar.ro/human3.6m/description.php}{``H36M''}. 
Regarding the NTU RGB+D dataset, please refer to \href{https://rose1.ntu.edu.sg/dataset/actionRecognition/}{``NTU RGB+D''}.
Regarding the H3WB dataset, please refer to \href{https://github.com/wholebody3d/wholebody3d}{``H3HB''}.
After downloading each dataset, for further dataset preparation steps, please refer to our \href{https://anonymous.4open.science/r/GTAutoAct-4CB6/README.md}{project repository}. 
This will provide the necessary guidance on how to properly configure and utilize the datasets for specific requirements.

\subsection{Model Configuration}
For detailed information on the configuration of each model used in our experiments, please refer to Section B.2. of the appendix. 
This section contains specific implementation details crucial for replicating or understanding our models' setups.
Alternatively, you can directly download the configuration file for each model from our \href{https://anonymous.4open.science/r/GTAutoAct-4CB6/README.md}{project repository}. 
Additionally, we have included several configuration files in the ``testing\_code/config'' directory. 
These files are intended to assist in setting up and running the tests efficiently, ensuring an accurately reproduction in our evaluation process.

\subsection{Checkpoint}
To facilitate easy reproduction of our results, we have provided the trained checkpoints for each model corresponding to each dataset on our \href{https://anonymous.4open.science/r/GTAutoAct-4CB6/README.md}{project repository}. 
This allows for straightforward replication and analysis of our experimental findings.

\subsection{Evaluation}
For evaluation purposes, you can either follow the official instruction file of MMAction or download our custom testing code, designed for batch processing on server or supercomputer systems. 
Additionally, we have included run files in the ``testing\_code/run\_file'' directory. 
This code is also available in our repository and is tailored for efficient, large-scale evaluation of the models.
